# Supplementary material for: Electrical Control of Optical Properties of Monolayer MoS$_2$
Source: arXiv:1211.0341 source file (2012-11-02)
Supplement: Supplementary file 1 [file supplementary_materials.pdf]

Supplementary Material

# Electrical Control of Optical Properties of Monolayer $MoS_2$

A.K.M. Newaz[a], D. Prasai[b], J.I. Ziegler[a], D. Caudel[a,c], S. Robinson[d], R.F. Haglund, Jr. [a,b], K.I. Bolotin[a,b]

[a]Department of Physics and Astronomy, Vanderbilt University, Nashville, Tennessee 37235-1807, USA,

[b] Interdisciplinary Graduate Program in Materials Science, Vanderbilt University, Nashville, Tennessee 37234-0106, USA,

[c] Department of Physics, Fisk University, Nashville, Tennessee 37208, USA

[d] Department of Chemistry and Physics, Belmont University, Nashville, Tennessee 37212, USA

## 1. Photoluminescence spectra for Device #3

The gate dependent PL data for the device #3 are presented in Fig. S1. The PL data were recorded for 1μW laser excitation power, with a spot size ~1 μm. The measured mobility of this device is $\mu$~1 cm$^2$/Vs.

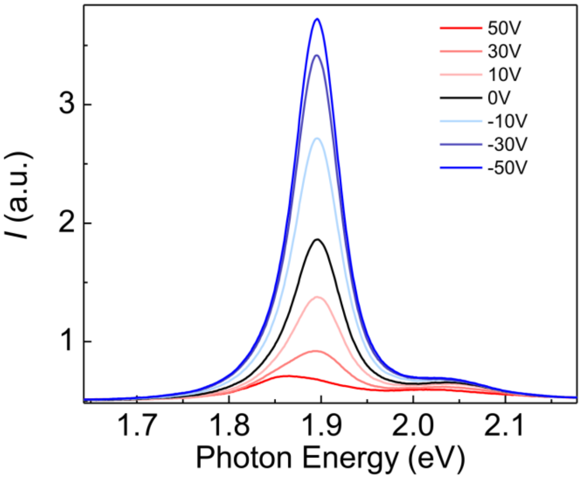


***Figure S1:*** *Gate dependent PL spectra for a monolayer $MoS_2$ device #3 at low excitation power (1μW). PL spectra were taken at different gate voltages ($V_G$=-50V, -30V, -10V, 0V, 10V, 30V and 50V).*

## 2. Gate dependence of photoluminescence spectra

Variation of the PL spectra with gate voltage recorded at higher excitation power (50 μW) for the device #2 is shown in Fig. S2. We observe *a decrease* in the variation of the PL intensity at high excitation power compared to the data at 1 μW (Fig. S1). We also found a decrease in the intensity of the normalized PL signal at a fixed gate voltage as we increased the laser excitation power in the range 1-200μW (Fig. S2, Inset). These data can be accounted for by either interaction between photoexcited excitons or simply by the effect of sample heating at large excitation power.

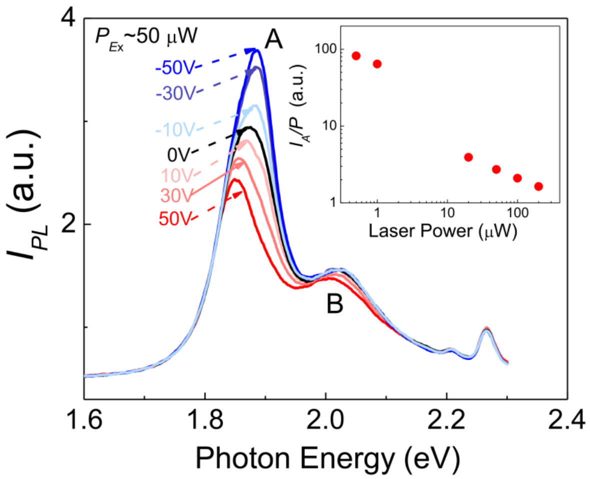


***Figure S2:*** *PL spectra for the device #2 in the range of gate voltages ($V_G$=-50V, -30V, -10V, 0V, 10V, 30V, 50V) at the excitation power 50 μW. The inset is showing the integrated intensity of "A" peak normalized to the excitation power, while the excitation power is varied in the range 0.5 - 200 μW.*

## 3. Dependence of photoluminescence intensity on sample mobility

We compared the PL data from 3 devices with mobility ranging from 1 to 13 $cm^2/Vs$. To extend the range of accessible carrier mobilities, we have also intentionally damaged one device by exposing it to ozone. The mobility of that device after 150s of ozone exposure (Jelight Company, Model-42) was 0.1 $cm^2/Vs$. Both conductivity and PL intensity for all of these devices are plotted as a function of $V_G$ in Fig. S3. While mobilities are varying over two orders of magnitude between these devices (Fig. S3a), $I_{PL}(V_G)$ curves are very similar with less than a factor of two variation of the PL intensity at $V_G$=-50V (Fig. S3b).

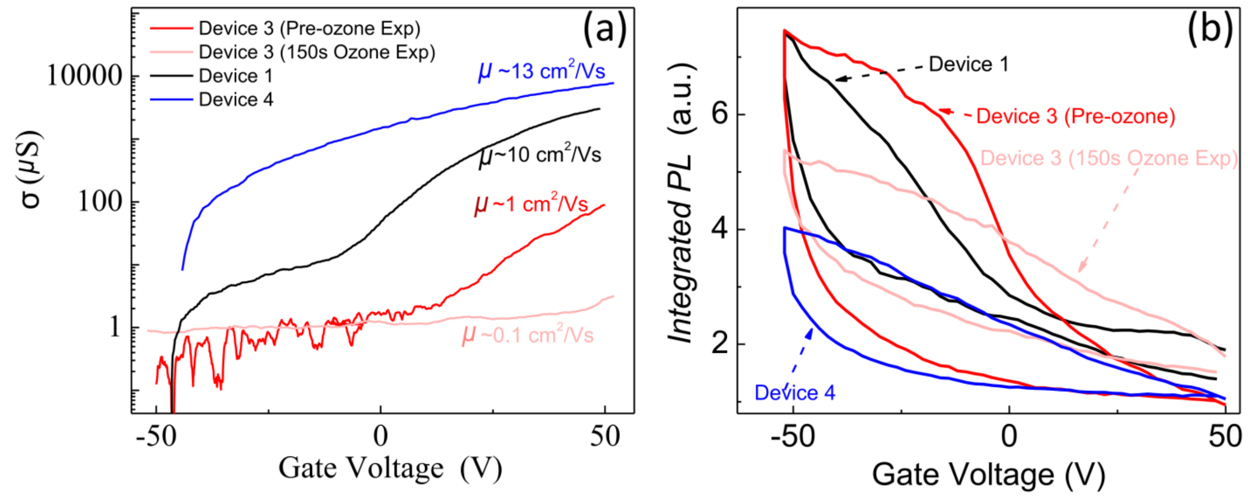


***Figure S3:*** *Mobility dependence of electrical and optical properties of monolayer $MoS_2$. a) The conductance data from 3 devices with differing mobility. The source drain voltage was kept at 50mV. b) Gate voltage dependence of the integrated photoluminescence intensity for the same set of devices. The excitation power was kept at 1 μW for all the measurements.*

## 4. Photocurrent in a monolayer $MoS_2$ FET

Typical $I_{ds}(V_G)$ curve for the Device #1 under illumination and in the dark is shown in Fig. S4.

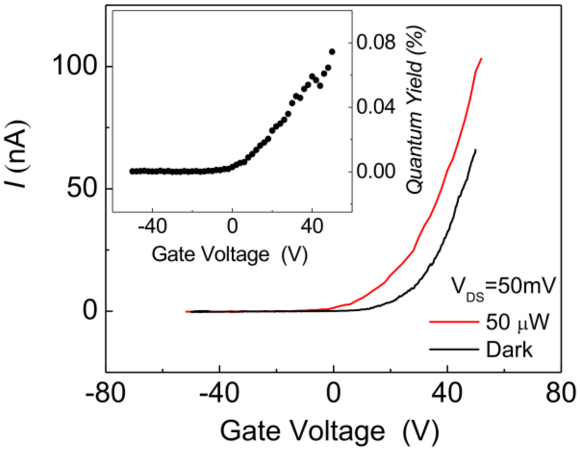


***Figure S4.*** *$I_{ds}(V_G)$ plot for the device #1 in the dark (black curve) and under 50 μW laser excitation (red curve). The inset is showing the calculated quantum efficiency for photocurrent.*

## 5. Gate dependence of PL spectra from a bilayer $MoS_2$

Variation of the PL spectra with gate voltage recorded at low excitation power (2 μW) for a bilayer $MoS_2$ FET device is shown in Fig. S5.

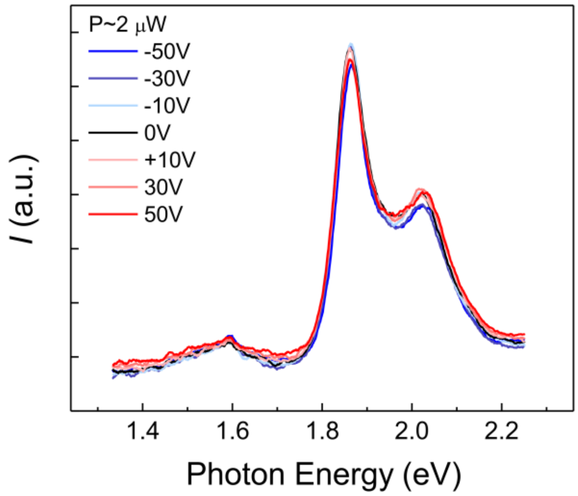


***Figure S5:*** *PL spectra for a bilayer device in the range of gate voltages ($V_G$=-50V, -30V, -10V, 0V, 10V, 30V, 50V) at the excitation power 2 μW.*
